# Supplementary material for: Vibrational Heat-Bath Configuration Interaction
Source: arXiv:2010.12123 ancillary file (2020-10-23)
Supplement: Supplementary file 1 [file VHCI_SI.pdf]

# Supplementary material: Vibrational heat-bath configuration interaction

Jonathan H. Fetherolf[1] and Timothy C. Berkelbach[1,2,a)]

[1)]*Department of Chemistry, Columbia University, New York, New York 10027, USA*

[2)]*Center for Computational Quantum Physics, Flatiron Institute, New York, New York 10010, USA*

[a)]Electronic mail: tim.berkelbach@gmail.com

## S1. ACETONITRILE

TABLE S1: 70 lowest-energy states of acetonitrile computed with VHCI and VHCI+PT2. Excited states are reported relative to the ZPE. Calculated using the quartic PES from Ref. 1. Multiple assignments are given when the CI wavefunction weight differs by less than a factor of two. Assignments use the mode-numbering convention of Ref. 2, and are taken from the $\varepsilon_1$ = 0.1 $cm^{-1}$ calculation. All energies are in $cm^{-1}$.

| | | $\varepsilon_1 = 1.0$ | | $\varepsilon_1 = 0.1$ | |
|---|---|---|---|---|---|
| | Assignment | Var | Full PT2 | Var | Full PT2 |
| 1 | ZPE | 9837.43 | 9837.41 | 9837.41 | 9837.41 |
| 2 | $0.97(\omega_{11})$ | 361.01 | 360.99 | 360.99 | 360.99 |
| 3 | $0.97(\omega_{12})$ | 361.01 | 360.99 | 360.99 | 360.99 |
| 4 | $0.97(\omega_{11}+\omega_{12})$ | 723.22 | 723.18 | 723.18 | 723.18 |
| 5 | $0.69(2\omega_{11})$, $0.69(2\omega_{12})$ | 723.25 | 723.19 | 723.18 | 723.18 |
| 6 | $0.68(2\omega_{11})$, $0.68(2\omega_{12})$ | 723.90 | 723.84 | 723.83 | 723.83 |
| 7 | $0.95(\omega_4)$ | 900.70 | 900.66 | 900.66 | 900.66 |
| 8 | $0.97(\omega_9)$ | 1034.18 | 1034.13 | 1034.13 | 1034.12 |
| 9 | $0.97(\omega_{10})$ | 1034.19 | 1034.13 | 1034.13 | 1034.12 |
| 10 | $0.84(\omega_{11}+2\omega_{12})$, $0.48(3\omega_{11})$ | 1086.65 | 1086.56 | 1086.56 | 1086.55 |
| 11 | $0.48(3\omega_{12})$, $0.84(2\omega_{11}+\omega_{12})$ | 1086.66 | 1086.56 | 1086.56 | 1086.55 |
| 12 | $0.48(\omega_{11}+2\omega_{12})$, $0.83(3\omega_{11})$ | 1087.88 | 1087.79 | 1087.78 | 1087.78 |
| 13 | $0.83(3\omega_{12})$, $0.48(2\omega_{11}+\omega_{12})$ | 1087.88 | 1087.79 | 1087.78 | 1087.78 |

| | | | | | |
|---|---|---|---|---|---|
| 14 | 0.94($\omega_4 + \omega_{11}$) | 1259.89 | 1259.82 | 1259.81 | 1259.81 |
| 15 | 0.94($\omega_4 + \omega_{12}$) | 1259.94 | 1259.83 | 1259.82 | 1259.81 |
| 16 | 0.73($\omega_3$),<br>0.45($\omega_9 + \omega_{11}$),<br>0.45($\omega_{10} + \omega_{12}$) | 1389.10 | 1388.99 | 1388.98 | 1388.97 |
| 17 | 0.68($\omega_{11} + \omega_{10}$),<br>0.68($\omega_9 + \omega_{12}$) | 1394.86 | 1394.71 | 1394.69 | 1394.68 |
| 18 | 0.68($\omega_9 + \omega_{11}$),<br>0.68($\omega_{10} + \omega_{12}$) | 1394.89 | 1394.71 | 1394.70 | 1394.68 |
| 19 | 0.68($\omega_{11} + \omega_{10}$),<br>0.68($\omega_9 + \omega_{12}$) | 1395.08 | 1394.93 | 1394.91 | 1394.90 |
| 20 | 0.64($\omega_3$),<br>0.51($\omega_9 + \omega_{11}$),<br>0.51($\omega_{10} + \omega_{12}$) | 1397.83 | 1397.70 | 1397.69 | 1397.68 |
| 21 | 0.84($2\omega_{11} + 2\omega_{12}$) | 1451.37 | 1451.13 | 1451.11 | 1451.10 |
| 22 | 0.68($3\omega_{11} + \omega_{12}$),<br>0.68($\omega_{11} + 3\omega_{12}$) | 1451.38 | 1451.13 | 1451.11 | 1451.10 |
| 23 | 0.68($4\omega_{11}$),<br>0.67($4\omega_{12}$) | 1453.14 | 1452.86 | 1452.84 | 1452.82 |
| 24 | 0.68($3\omega_{11} + \omega_{12}$),<br>0.68($\omega_{11} + 3\omega_{12}$) | 1453.16 | 1452.87 | 1452.84 | 1452.82 |
| 25 | 0.58($4\omega_{11}$),<br>0.48($2\omega_{11} + 2\omega_{12}$),<br>0.59($4\omega_{12}$) | 1453.76 | 1453.44 | 1453.42 | 1453.40 |
| 26 | 0.97($\omega_7$) | 1483.28 | 1483.23 | 1483.23 | 1483.22 |
| 27 | 0.97($\omega_8$) | 1483.29 | 1483.23 | 1483.23 | 1483.22 |
| 28 | 0.93($\omega_4 + \omega_{11} + \omega_{12}$) | 1620.47 | 1620.25 | 1620.21 | 1620.20 |
| 29 | 0.66($\omega_4 + 2\omega_{12}$),<br>0.66($\omega_4 + 2\omega_{11}$) | 1620.58 | 1620.27 | 1620.22 | 1620.20 |

| | | | | | |
|---|---|---|---|---|---|
| 30 | $0.66(\omega_4 + 2\omega_{12})$, $0.65(\omega_4 + 2\omega_{11})$ | 1621.14 | 1620.81 | 1620.77 | 1620.74 |
| 31 | $0.74(\omega_3 + \omega_{11})$, $0.50(\omega_9 + 2\omega_{11})$ | 1749.74 | 1749.55 | 1749.54 | 1749.52 |
| 32 | $0.74(\omega_3 + \omega_{12})$, $0.50(\omega_{10} + 2\omega_{12})$ | 1749.74 | 1749.55 | 1749.54 | 1749.52 |
| 33 | $0.48(\omega_{10} + 2\omega_{12})$, $0.68(\omega_9 + \omega_{11} + \omega_{12})$, $0.48(2\omega_{11} + \omega_{10})$ | 1756.67 | 1756.45 | 1756.44 | 1756.42 |
| 34 | $0.68(\omega_{11} + \omega_{10} + \omega_{12})$, $0.48(\omega_9 + 2\omega_{11})$, $0.48(\omega_9 + 2\omega_{12})$ | 1756.68 | 1756.45 | 1756.44 | 1756.42 |
| 35 | $0.83(2\omega_{11} + \omega_{10})$ | 1757.37 | 1757.16 | 1757.14 | 1757.12 |
| 36 | $0.83(\omega_9 + 2\omega_{12})$ | 1757.38 | 1757.16 | 1757.14 | 1757.12 |
| 37 | $0.62(\omega_3 + \omega_{11})$, $0.42(\omega_{11} + \omega_{10} + \omega_{12})$, $0.60(\omega_9 + 2\omega_{11})$ | 1760.00 | 1759.79 | 1759.78 | 1759.76 |
| 38 | $0.62(\omega_3 + \omega_{12})$, $0.60(\omega_{10} + 2\omega_{12})$, $0.42(\omega_9 + \omega_{11} + \omega_{12})$ | 1760.00 | 1759.79 | 1759.78 | 1759.76 |
| 39 | $0.89(2\omega_4)$ | 1785.64 | 1785.24 | 1785.12 | 1785.10 |
| 40 | $0.54(4\omega_{11} + \omega_{12})$, $0.76(2\omega_{11} + 3\omega_{12})$ | 1817.22 | 1816.84 | 1816.82 | 1816.79 |
| 41 | $0.54(\omega_{11} + 4\omega_{12})$, $0.76(3\omega_{11} + 2\omega_{12})$ | 1817.23 | 1816.85 | 1816.82 | 1816.79 |
| 42 | $0.53(5\omega_{11})$, $0.71(\omega_{11} + 4\omega_{12})$ | 1819.44 | 1819.01 | 1818.98 | 1818.94 |
| 43 | $0.53(5\omega_{12})$, $0.71(4\omega_{11} + \omega_{12})$ | 1819.53 | 1819.02 | 1818.98 | 1818.94 |

| | | | | | |
|---|---|---|---|---|---|
| 44 | $0.75(5\omega_{12})$, $0.47(2\omega_{11} + 3\omega_{12})$ | 1820.55 | 1820.09 | 1820.05 | 1820.02 |
| 45 | $0.75(5\omega_{11})$, $0.47(3\omega_{11} + 2\omega_{12})$ | 1820.63 | 1820.10 | 1820.05 | 1820.02 |
| 46 | $0.67(\omega_{11} + \omega_8)$, $0.69(\omega_7 + \omega_{12})$ | 1844.40 | 1844.26 | 1844.26 | 1844.25 |
| 47 | $0.70(\omega_{11} + \omega_8)$, $0.67(\omega_7 + \omega_{12})$ | 1844.47 | 1844.34 | 1844.33 | 1844.32 |
| 48 | $0.69(\omega_7 + \omega_{11})$, $0.68(\omega_8 + \omega_{12})$ | 1844.52 | 1844.34 | 1844.33 | 1844.32 |
| 49 | $0.68(\omega_7 + \omega_{11})$, $0.69(\omega_8 + \omega_{12})$ | 1844.87 | 1844.70 | 1844.69 | 1844.68 |
| 50 | $0.94(\omega_4 + \omega_9)$ | 1931.80 | 1931.57 | 1931.53 | 1931.52 |
| 51 | $0.94(\omega_4 + \omega_{10})$ | 1931.83 | 1931.57 | 1931.54 | 1931.52 |
| 52 | $0.80(\omega_4 + \omega_{11} + 2\omega_{12})$, $0.46(\omega_4 + 3\omega_{11})$ | 1982.24 | 1981.89 | 1981.84 | 1981.82 |
| 53 | $0.46(\omega_4 + 3\omega_{12})$, $0.80(\omega_4 + 2\omega_{11} + \omega_{12})$ | 1982.27 | 1981.89 | 1981.84 | 1981.82 |
| 54 | $0.45(\omega_4 + \omega_{11} + 2\omega_{12})$, $0.78(\omega_4 + 3\omega_{11})$ | 1983.27 | 1982.90 | 1982.85 | 1982.82 |
| 55 | $0.79(\omega_4 + 3\omega_{12})$, $0.45(\omega_4 + 2\omega_{11} + \omega_{12})$ | 1983.32 | 1982.91 | 1982.85 | 1982.82 |
| 56 | $0.68(2\omega_9)$, $0.68(2\omega_{10})$ | 2057.48 | 2057.12 | 2057.08 | 2057.05 |
| 57 | $0.96(\omega_9 + \omega_{10})$ | 2065.57 | 2065.32 | 2065.29 | 2065.27 |
| 58 | $0.68(2\omega_9)$, $0.68(2\omega_{10})$ | 2065.61 | 2065.32 | 2065.29 | 2065.27 |
| 59 | $0.75(\omega_3 + \omega_{11} + \omega_{12})$, $0.43(\omega_9 + 2\omega_{11} + \omega_{12})$, $0.43(\omega_{11} + \omega_{10} + 2\omega_{12})$ | 2111.72 | 2111.42 | 2111.40 | 2111.37 |

| | | | | | |
|---|---|---|---|---|---|
| 60 | $0.35(\omega_9 + 3\omega_{11})$, $0.53(\omega_3 + 2\omega_{12})$, $0.35(\omega_{10} + 3\omega_{12})$, $0.53(\omega_3 + 2\omega_{11})$ | 2111.81 | 2111.43 | 2111.40 | 2111.37 |
| 61 | $0.37(\omega_9 + 3\omega_{11})$, $0.53(\omega_3 + 2\omega_{12})$, $0.37(\omega_{10} + 3\omega_{12})$, $0.53(\omega_3 + 2\omega_{11})$ | 2112.74 | 2112.35 | 2112.32 | 2112.29 |
| 62 | $0.34(3\omega_{11} + \omega_{10})$, $0.59(\omega_9 + 2\omega_{11} + \omega_{12})$, $0.59(\omega_{11} + \omega_{10} + 2\omega_{12})$, $0.34(\omega_9 + 3\omega_{12})$ | 2119.75 | 2119.38 | 2119.35 | 2119.31 |
| 63 | $0.34(\omega_9 + 3\omega_{11})$, $0.59(2\omega_{11} + \omega_{10} + \omega_{12})$, $0.34(\omega_{10} + 3\omega_{12})$, $0.59(\omega_9 + \omega_{11} + 2\omega_{12})$ | 2119.83 | 2119.38 | 2119.36 | 2119.31 |
| 64 | $0.67(3\omega_{11} + \omega_{10})$, $0.68(\omega_9 + 3\omega_{12})$ | 2120.96 | 2120.59 | 2120.56 | 2120.53 |
| 65 | $0.36(\omega_9 + 3\omega_{11})$, $0.57(2\omega_{11} + \omega_{10} + \omega_{12})$, $0.36(\omega_{10} + 3\omega_{12})$, $0.57(\omega_9 + \omega_{11} + 2\omega_{12})$ | 2121.08 | 2120.61 | 2120.57 | 2120.53 |
| 66 | $0.59(3\omega_{11} + \omega_{10})$, $0.34(\omega_9 + 2\omega_{11} + \omega_{12})$, $0.34(\omega_{11} + \omega_{10} + 2\omega_{12})$, $0.58(\omega_9 + 3\omega_{12})$ | 2121.36 | 2120.96 | 2120.93 | 2120.90 |
| 67 | $0.61(\omega_3 + \omega_{11} + \omega_{12})$, $0.52(\omega_9 + 2\omega_{11} + \omega_{12})$, $0.52(\omega_{11} + \omega_{10} + 2\omega_{12})$ | 2123.24 | 2122.88 | 2122.86 | 2122.82 |

| | | | | | |
|---|---|---|---|---|---|
| 68 | $0.45(\omega_9 + 3\omega_{11})$, $0.27(2\omega_{11} + \omega_{10} + \omega_{12})$, $0.43(\omega_3 + 2\omega_{12})$, $0.45(\omega_{10} + 3\omega_{12})$, $0.43(\omega_3 + 2\omega_{11})$, $0.26(\omega_9 + \omega_{11} + 2\omega_{12})$ | 2123.32 | 2122.89 | 2122.86 | 2122.82 |
| 69 | $0.45(\omega_9 + 3\omega_{11})$, $0.26(2\omega_{11} + \omega_{10} + \omega_{12})$, $0.43(\omega_3 + 2\omega_{12})$, $0.46(\omega_{10} + 3\omega_{12})$, $0.42(\omega_3 + 2\omega_{11})$, $0.26(\omega_9 + \omega_{11} + 2\omega_{12})$ | 2123.83 | 2123.36 | 2123.33 | 2123.29 |
| 70 | $0.87(2\omega_4 + \omega_{11})$ | 2142.90 | 2142.48 | 2142.38 | 2142.36 |

## S2. ETHYLENE

TABLE S2: 100 lowest-energy states of ethylene computed with VHCI+PT2. Excited states are reported relative to the ZPE. Calculated with the quartic and sextic PES from Ref. 3 and 4. Multiple assignments are given when the CI wavefunction weight differs by less than a factor of two. Assignments use the mode-numbering convention of Ref. 3 and are taken from the 6th-order PES calculation. All energies are in $cm^{-1}$.

| | Assignment | 4th-order $\varepsilon_1 = 0.75$ Full PT2 | 6th-order $\varepsilon_1 = 0.5$ $\varepsilon_2 = 0.01$ |
|---|---|---|---|
| 1 | ZPE | 11006.11 | 11011.61 |
| 2 | $0.98(\omega_{10})$ | 808.61 | 819.99 |
| 3 | $0.98(\omega_8)$ | 914.87 | 926.33 |

| | | | |
|---|---|---|---|
| 4 | $0.98(\omega_7)$ | 927.87 | 941.65 |
| 5 | $0.98(\omega_4)$ | 1006.74 | 1017.45 |
| 6 | $0.98(\omega_6)$ | 1216.94 | 1222.16 |
| 7 | $0.97(\omega_3)$ | 1338.46 | 1341.95 |
| 8 | $0.98(\omega_{12})$ | 1429.93 | 1438.31 |
| 9 | $0.87(\omega_2)$ | 1606.41 | 1622.78 |
| 10 | $0.88(2\omega_{10})$ | 1631.47 | 1655.21 |
| 11 | $0.98(\omega_{10} + \omega_8)$ | 1718.27 | 1748.05 |
| 12 | $0.98(\omega_{10} + \omega_7)$ | 1733.98 | 1766.19 |
| 13 | $0.98(\omega_{10} + \omega_4)$ | 1809.39 | 1837.68 |
| 14 | $0.97(2\omega_8)$ | 1821.71 | 1858.36 |
| 15 | $0.97(\omega_8 + \omega_7)$ | 1821.96 | 1871.42 |
| 16 | $0.97(2\omega_7)$ | 1850.39 | 1887.03 |
| 17 | $0.97(\omega_8 + \omega_4)$ | 1898.13 | 1939.47 |
| 18 | $0.97(\omega_7 + \omega_4)$ | 1907.64 | 1953.05 |
| 19 | $0.98(2\omega_4)$ | 2004.32 | 2032.09 |
| 20 | $0.97(\omega_{10} + \omega_6)$ | 2008.52 | 2037.42 |
| 21 | $0.98(\omega_8 + \omega_6)$ | 2131.63 | 2150.22 |
| 22 | $0.96(\omega_{10} + \omega_3)$ | 2143.44 | 2164.52 |
| 23 | $0.98(\omega_7 + \omega_6)$ | 2144.13 | 2165.70 |
| 24 | $0.98(\omega_4 + \omega_6)$ | 2220.53 | 2239.78 |
| 25 | $0.97(\omega_{10} + \omega_{12})$ | 2223.60 | 2256.14 |
| 26 | $0.97(\omega_8 + \omega_3)$ | 2247.64 | 2265.29 |
| 27 | $0.97(\omega_7 + \omega_3)$ | 2261.20 | 2281.61 |
| 28 | $0.97(\omega_4 + \omega_3)$ | 2334.33 | 2355.60 |
| 29 | $0.97(\omega_8 + \omega_{12})$ | 2339.50 | 2362.05 |
| 30 | $0.97(\omega_7 + \omega_{12})$ | 2343.43 | 2375.37 |
| 31 | $0.89(\omega_{10} + \omega_2)$ | 2390.43 | 2433.40 |
| 32 | $0.98(2\omega_6)$ | 2430.00 | 2443.25 |
| 33 | $0.98(\omega_4 + \omega_{12})$ | 2430.83 | 2454.55 |

| | | | |
|---|---|---|---|
| 34 | $0.89(3\omega_{10})$ | 2435.40 | 2496.84 |
| 35 | $0.91(\omega_8 + \omega_2)$ | 2508.37 | 2543.21 |
| 36 | $0.92(\omega_7 + \omega_2)$ | 2524.96 | 2560.06 |
| 37 | $0.96(\omega_6 + \omega_3)$ | 2526.37 | 2561.77 |
| 38 | $0.92(2\omega_{10} + \omega_8)$ | 2537.01 | 2583.60 |
| 39 | $0.93(2\omega_{10} + \omega_7)$ | 2549.09 | 2604.16 |
| 40 | $0.89(\omega_4 + \omega_2)$ | 2598.57 | 2637.04 |
| 41 | $0.97(\omega_6 + \omega_{12})$ | 2611.25 | 2654.69 |
| 42 | $0.90(2\omega_{10} + \omega_4)$ | 2615.18 | 2672.59 |
| 43 | $0.95(2\omega_3)$ | 2621.46 | 2682.09 |
| 44 | $0.97(\omega_{10} + 2\omega_8)$ | 2636.21 | 2682.25 |
| 45 | $0.96(\omega_{10} + \omega_8 + \omega_7)$ | 2652.05 | 2698.18 |
| 46 | $0.97(\omega_{10} + 2\omega_7)$ | 2674.40 | 2716.52 |
| 47 | $0.97(\omega_{10} + \omega_8 + \omega_4)$ | 2667.93 | 2762.07 |
| 48 | $0.96(\omega_3 + \omega_{12})$ | 2668.27 | 2774.81 |
| 49 | $0.97(\omega_{10} + \omega_7 + \omega_4)$ | 2685.63 | 2778.47 |
| 50 | $0.95(3\omega_8)$ | 2697.32 | 2795.74 |
| 51 | $0.94(2\omega_8 + \omega_7)$ | 2726.98 | 2807.43 |
| 52 | $0.93(\omega_8 + 2\omega_7)$ | 2732.64 | 2822.82 |
| 53 | $0.89(\omega_6 + \omega_2)$ | 2746.19 | 2830.62 |
| 54 | $0.94(3\omega_7)$ | 2758.89 | 2837.07 |
| 55 | $0.97(\omega_{10} + 2\omega_4)$ | 2758.64 | 2852.89 |
| 56 | $0.91(2\omega_{10} + \omega_6)$ | 2779.24 | 2867.00 |
| 57 | $0.95(2\omega_8 + \omega_4)$ | 2798.59 | 2868.34 |
| 58 | $0.95(2\omega_{12})$ | 2802.34 | 2869.49 |
| 59 | $0.95(\omega_8 + \omega_7 + \omega_4)$ | 2825.86 | 2882.36 |
| 60 | $0.94(2\omega_7 + \omega_4)$ | 2848.45 | 2894.74 |
| 61 | $0.96(\omega_8 + 2\omega_4)$ | 2862.04 | 2951.20 |
| 62 | $0.88(\omega_3 + \omega_2)$ | 2868.70 | 2957.37 |
| 63 | $0.95(\omega_7 + 2\omega_4)$ | 2915.27 | 2963.24 |

| | | | |
|---|---|---|---|
| 64 | $0.97(\omega_{10} + \omega_8 + \omega_6)$ | 2925.63 | 2967.92 |
| 65 | $0.86(\omega_{11})$ | 2930.37 | 2978.02 |
| 66 | $0.97(\omega_{10} + \omega_7 + \omega_6)$ | 2957.83 | 2986.11 |
| 67 | $0.86(2\omega_{10} + \omega_3)$ | 2975.62 | 2999.66 |
| 68 | $0.85(\omega_1)$ | 2989.97 | 3016.73 |
| 69 | $0.97(3\omega_4)$ | 2994.25 | 3044.12 |
| 70 | $0.97(\omega_{10} + \omega_4 + \omega_6)$ | 3000.64 | 3055.54 |
| 71 | $0.66(\omega_{12} + \omega_2)$, $0.61(2\omega_{10} + \omega_{12})$ | 3020.15 | 3070.16 |
| 72 | $0.87(\omega_5)$ | 3032.01 | 3071.18 |
| 73 | $0.92(2\omega_8 + \omega_6)$ | 3033.64 | 3084.99 |
| 74 | $0.96(\omega_{10} + \omega_8 + \omega_3)$ | 3044.66 | 3089.95 |
| 75 | $0.80(\omega_9)$, $0.50(\omega_8 + \omega_7 + \omega_6)$ | 3061.40 | 3091.40 |
| 76 | $0.56(\omega_{12} + \omega_2)$, $0.73(2\omega_{10} + \omega_{12})$ | 3065.16 | 3095.72 |
| 77 | $0.47(\omega_9)$, $0.82(\omega_8 + \omega_7 + \omega_6)$ | 3066.86 | 3099.48 |
| 78 | $0.96(\omega_{10} + \omega_7 + \omega_3)$ | 3077.86 | 3109.05 |
| 79 | $0.97(2\omega_7 + \omega_6)$ | 3097.91 | 3113.19 |
| 80 | $0.97(\omega_8 + \omega_4 + \omega_6)$ | 3105.98 | 3163.68 |
| 81 | $0.97(\omega_7 + \omega_4 + \omega_6)$ | 3113.36 | 3177.55 |
| 82 | $0.95(\omega_{10} + \omega_4 + \omega_3)$ | 3118.62 | 3178.70 |
| 83 | $0.96(\omega_{10} + \omega_8 + \omega_{12})$ | 3130.12 | 3182.15 |
| 84 | $0.96(2\omega_8 + \omega_3)$ | 3136.12 | 3194.44 |
| 85 | $0.96(\omega_{10} + \omega_7 + \omega_{12})$ | 3137.84 | 3198.54 |
| 86 | $0.96(\omega_8 + \omega_7 + \omega_3)$ | 3138.18 | 3208.87 |
| 87 | $0.96(2\omega_7 + \omega_3)$ | 3152.07 | 3225.33 |
| 88 | $0.68(2\omega_2)$, $0.60(2\omega_{10} + \omega_2)$ | 3175.80 | 3235.82 |

| | | | |
|---|---|---|---|
| 89 | $0.96(\omega_{10} + 2\omega_6)$ | 3195.91 | 3254.54 |
| 90 | $0.97(2\omega_4 + \omega_6)$ | 3194.82 | 3254.64 |
| 91 | $0.61(2\omega_2)$, $0.65(2\omega_{10} + \omega_2)$ | 3199.22 | 3269.63 |
| 92 | $0.97(\omega_{10} + \omega_4 + \omega_{12})$ | 3211.86 | 3273.12 |
| 93 | $0.96(\omega_8 + \omega_4 + \omega_3)$ | 3214.89 | 3274.71 |
| 94 | $0.96(\omega_7 + \omega_4 + \omega_3)$ | 3218.48 | 3289.42 |
| 95 | $0.96(2\omega_8 + \omega_{12})$ | 3221.81 | 3291.89 |
| 96 | $0.95(\omega_8 + \omega_7 + \omega_{12})$ | 3233.27 | 3304.09 |
| 97 | $0.95(2\omega_7 + \omega_{12})$ | 3250.26 | 3317.19 |
| 98 | $0.87(4\omega_{10})$ | 3253.29 | 3348.99 |
| 99 | $0.91(\omega_{10} + \omega_8 + \omega_2)$ | 3276.78 | 3355.81 |
| 100 | $0.96(2\omega_4 + \omega_3)$ | 3298.16 | 3366.39 |

## S3. ETHYLENE OXIDE

TABLE S3: 200 lowest-energy states of ethylene oxide computed with VHCI and VHCI+PT2. Excited states are reported relative to the ZPE. Calculated using the quartic PES from Ref. 5. Multiple assignments are given when the CI wavefunction weight differs by less than a factor of two. Assignments use the mode-numbering convention of Ref. 6 and are taken from the $\varepsilon_1 = 1$ cm$^{-1}$ calculation, while the $\varepsilon_1 = 2$ cm$^{-1}$ data is presented in order of energy. All energies are in cm$^{-1}$.

| | | $\varepsilon_1 = 2$ | | $\varepsilon_1 = 1$ | | Extrap. |
|---|---|---|---|---|---|---|
| | Assignment | Var | $\varepsilon_2 = 0.01$ | Var | $\varepsilon_2 = 0.01$ | $\varepsilon_2 = 0.01$ |
| 1 | ZPE | 12461.63 | 12461.50 | 12461.55 | 12461.48 | 12461.47 |
| 2 | $0.97(\omega_1)$ | 793.11 | 792.73 | 792.88 | 792.69 | 792.65 |
| 3 | $0.96(\omega_2)$ | 822.30 | 821.98 | 822.07 | 821.94 | 821.91 |
| 4 | $0.97(\omega_3)$ | 878.62 | 878.33 | 878.41 | 878.30 | 878.28 |

| | | | | | | |
|---|---|---|---|---|---|---|
| 5 | $0.97(\omega_4)$ | 1017.70 | 1017.24 | 1017.42 | 1017.20 | 1017.15 |
| 6 | $0.96(\omega_6)$ | 1121.87 | 1121.30 | 1121.53 | 1121.24 | 1121.19 |
| 7 | $0.97(\omega_5)$ | 1124.37 | 1123.75 | 1124.00 | 1123.70 | 1123.65 |
| 8 | $0.97(\omega_7)$ | 1146.42 | 1145.84 | 1146.08 | 1145.78 | 1145.73 |
| 9 | $0.97(\omega_8)$ | 1148.68 | 1148.07 | 1148.31 | 1148.02 | 1147.97 |
| 10 | $0.94(\omega_9)$ | 1271.43 | 1270.89 | 1271.06 | 1270.83 | 1270.78 |
| 11 | $0.97(\omega_{10})$ | 1468.28 | 1467.49 | 1467.81 | 1467.42 | 1467.34 |
| 12 | $0.94(\omega_{11})$ | 1496.22 | 1495.35 | 1495.68 | 1495.26 | 1495.17 |
| 13 | $0.94(2\omega_1)$ | 1588.85 | 1587.50 | 1588.00 | 1587.31 | 1587.12 |
| 14 | $0.96(\omega_1 + \omega_2)$ | 1612.77 | 1611.29 | 1611.79 | 1611.10 | 1610.93 |
| 15 | $0.92(2\omega_2)$ | 1642.78 | 1641.28 | 1641.58 | 1641.04 | 1640.90 |
| 16 | $0.96(\omega_3 + \omega_1)$ | 1672.17 | 1670.53 | 1671.17 | 1670.36 | 1670.18 |
| 17 | $0.94(\omega_3 + \omega_2)$ | 1696.56 | 1695.20 | 1695.60 | 1695.02 | 1694.88 |
| 18 | $0.94(2\omega_3)$ | 1756.09 | 1754.90 | 1755.32 | 1754.75 | 1754.63 |
| 19 | $0.96(\omega_4 + \omega_1)$ | 1808.05 | 1805.87 | 1806.81 | 1805.61 | 1805.28 |
| 20 | $0.94(\omega_4 + \omega_2)$ | 1834.73 | 1832.62 | 1833.32 | 1832.34 | 1832.09 |
| 21 | $0.92(\omega_3 + \omega_4)$ | 1891.26 | 1889.32 | 1890.04 | 1889.09 | 1888.87 |
| 22 | $0.91(\omega_1 + \omega_5)$ | 1909.36 | 1907.19 | 1908.18 | 1906.94 | 1906.61 |
| 23 | $0.93(\omega_6 + \omega_1)$ | 1911.33 | 1909.15 | 1910.02 | 1908.87 | 1908.55 |
| 24 | $0.82(\omega_8 + \omega_1)$,<br>$0.46(\omega_6 + \omega_2)$ | 1930.04 | 1927.71 | 1928.58 | 1927.39 | 1927.05 |
| 25 | $0.86(\omega_7 + \omega_1)$ | 1939.91 | 1937.81 | 1938.58 | 1937.53 | 1937.26 |
| 26 | $0.48(\omega_8 + \omega_1)$,<br>$0.81(\omega_6 + \omega_2)$ | 1941.54 | 1939.46 | 1940.11 | 1939.15 | 1938.89 |
| 27 | $0.43(\omega_7 + \omega_1)$,<br>$0.85(\omega_5 + \omega_2)$ | 1945.63 | 1943.62 | 1944.30 | 1943.36 | 1943.13 |
| 28 | $0.94(\omega_7 + \omega_2)$ | 1963.70 | 1961.60 | 1962.19 | 1961.28 | 1961.05 |
| 29 | $0.96(\omega_8 + \omega_2)$ | 1972.36 | 1970.32 | 1971.02 | 1970.06 | 1969.82 |
| 30 | $0.95(\omega_6 + \omega_3)$ | 1998.86 | 1997.06 | 1997.66 | 1996.83 | 1996.64 |
| 31 | $0.96(\omega_3 + \omega_5)$ | 2000.79 | 1998.79 | 1999.55 | 1998.55 | 1998.31 |

| | | | | | | |
|---|---|---|---|---|---|---|
| 32 | $0.96(\omega_3 + \omega_7)$ | 2022.68 | 2020.80 | 2021.52 | 2020.58 | 2020.35 |
| 33 | $0.96(\omega_3 + \omega_8)$ | 2025.63 | 2023.75 | 2024.44 | 2023.51 | 2023.29 |
| 34 | $0.96(2\omega_4)$ | 2033.68 | 2031.55 | 2032.38 | 2031.27 | 2030.96 |
| 35 | $0.93(\omega_9 + \omega_1)$ | 2062.34 | 2060.28 | 2061.00 | 2060.00 | 2059.74 |
| 36 | $0.91(\omega_9 + \omega_2)$ | 2087.96 | 2086.27 | 2086.82 | 2086.03 | 2085.82 |
| 37 | $0.92(\omega_6 + \omega_4)$ | 2129.67 | 2127.39 | 2128.30 | 2127.10 | 2126.79 |
| 38 | $0.93(\omega_4 + \omega_5)$ | 2136.22 | 2133.83 | 2134.82 | 2133.53 | 2133.18 |
| 39 | $0.90(\omega_9 + \omega_3)$ | 2142.10 | 2140.56 | 2141.10 | 2140.35 | 2140.15 |
| 40 | $0.92(\omega_4 + \omega_7)$ | 2154.17 | 2151.67 | 2152.63 | 2151.34 | 2150.99 |
| 41 | $0.96(\omega_8 + \omega_4)$ | 2167.03 | 2164.79 | 2165.72 | 2164.51 | 2164.19 |
| 42 | $0.84(2\omega_6)$ | 2235.66 | 2232.85 | 2233.90 | 2232.44 | 2231.99 |
| 43 | $0.91(\omega_6 + \omega_5)$ | 2242.35 | 2239.99 | 2240.94 | 2239.69 | 2239.35 |
| 44 | $0.83(\omega_1 + \omega_{10})$ | 2248.95 | 2246.10 | 2247.19 | 2245.70 | 2245.26 |
| 45 | $0.87(2\omega_5)$ | 2249.88 | 2247.66 | 2248.55 | 2247.39 | 2247.10 |
| 46 | $0.55(\omega_{11} + \omega_1)$, $0.69(\omega_8 + \omega_5)$ | 2266.73 | 2263.70 | 2264.81 | 2263.22 | 2262.70 |
| 47 | $0.90(\omega_6 + \omega_7)$ | 2268.96 | 2266.32 | 2267.32 | 2266.03 | 2265.76 |
| 48 | $0.85(\omega_7 + \omega_5)$ | 2268.98 | 2266.38 | 2267.37 | 2266.04 | 2265.69 |
| 49 | $0.85(\omega_6 + \omega_8)$, $0.43(\omega_1 + \omega_{10})$ | 2276.25 | 2273.77 | 2274.70 | 2273.47 | 2273.17 |
| 50 | $0.68(\omega_{11} + \omega_1)$, $0.63(\omega_8 + \omega_5)$ | 2285.11 | 2282.12 | 2283.30 | 2281.73 | 2281.28 |
| 51 | $0.89(\omega_{10} + \omega_2)$ | 2290.31 | 2288.12 | 2288.98 | 2287.82 | – |
| 52 | $0.84(\omega_9 + \omega_4)$ | 2291.60 | 2289.32 | 2290.11 | 2289.01 | – |
| 53 | $0.84(2\omega_7)$ | 2291.97 | 2289.62 | 2290.52 | 2289.34 | – |
| 54 | $0.96(\omega_8 + \omega_7)$ | 2294.77 | 2292.41 | 2293.38 | 2292.13 | – |
| 55 | $0.91(2\omega_8)$ | 2297.13 | 2294.98 | 2295.84 | 2294.72 | – |
| 56 | $0.90(\omega_{11} + \omega_2)$ | 2313.11 | 2310.71 | 2311.59 | 2310.35 | – |
| 57 | $0.96(\omega_3 + \omega_{10})$ | 2347.29 | 2345.33 | 2346.17 | 2345.10 | – |
| 58 | $0.90(\omega_{11} + \omega_3)$ | 2372.34 | 2370.22 | 2371.05 | 2369.93 | – |

| | | | | | | |
|---|---|---|---|---|---|---|
| 59 | $0.88(3\omega_1)$ | 2383.81 | 2379.56 | 2381.40 | 2378.83 | – |
| 60 | $0.90(\omega_9 + \omega_6)$ | 2390.83 | 2388.58 | 2389.31 | 2388.24 | – |
| 61 | $0.92(\omega_9 + \omega_5)$ | 2392.53 | 2390.22 | 2391.08 | 2389.92 | – |
| 62 | $0.92(2\omega_1 + \omega_2)$ | 2406.07 | 2402.11 | 2403.70 | 2401.41 | – |
| 63 | $0.92(\omega_9 + \omega_7)$ | 2416.82 | 2414.55 | 2415.39 | 2414.25 | – |
| 64 | $0.93(\omega_9 + \omega_8)$ | 2417.69 | 2415.42 | 2416.23 | 2415.12 | – |
| 65 | $0.90(\omega_1 + 2\omega_2)$ | 2432.43 | 2428.42 | 2429.82 | 2427.71 | – |
| 66 | $0.85(3\omega_2)$ | 2461.73 | 2458.33 | 2459.23 | 2457.58 | – |
| 67 | $0.93(\omega_3 + 2\omega_1)$ | 2467.95 | 2464.60 | 2466.08 | 2464.12 | – |
| 68 | $0.96(\omega_4 + \omega_{10})$ | 2483.60 | 2480.98 | 2482.00 | 2480.64 | – |
| 69 | $0.93(\omega_3 + \omega_1 + \omega_2)$ | 2487.76 | 2484.07 | 2485.52 | 2483.52 | – |
| 70 | $0.92(\omega_{11} + \omega_4)$ | 2509.14 | 2506.38 | 2507.52 | 2506.01 | – |
| 71 | $0.87(\omega_3 + 2\omega_2)$ | 2513.68 | 2510.38 | 2511.29 | 2509.70 | – |
| 72 | $0.88(2\omega_9)$ | 2538.86 | 2537.03 | 2537.72 | 2536.77 | – |
| 73 | $0.94(2\omega_3 + \omega_1)$ | 2549.89 | 2546.62 | 2547.99 | 2546.19 | – |
| 74 | $0.91(2\omega_3 + \omega_2)$ | 2570.38 | 2567.30 | 2568.38 | 2566.80 | – |
| 75 | $0.93(\omega_6 + \omega_{10})$ | 2585.73 | 2582.98 | 2584.07 | 2582.59 | – |
| 76 | $0.92(\omega_{10} + \omega_5)$ | 2589.52 | 2586.84 | 2587.94 | 2586.46 | – |
| 77 | $0.90(\omega_4 + 2\omega_1)$ | 2598.63 | 2593.79 | 2595.81 | 2592.91 | – |
| 78 | $0.85(\omega_7 + \omega_{10})$ | 2602.07 | 2599.09 | 2600.14 | 2598.68 | – |
| 79 | $0.86(\omega_8 + \omega_{10})$ | 2603.90 | 2601.12 | 2602.17 | 2600.74 | – |
| 80 | $0.81(\omega_{11} + \omega_6)$ | 2614.52 | 2611.55 | 2612.62 | 2610.99 | – |
| 81 | $0.90(\omega_{11} + \omega_5)$ | 2618.24 | 2615.42 | 2616.58 | 2615.04 | – |
| 82 | $0.86(\omega_4 + \omega_1 + \omega_2)$ | 2621.26 | 2616.36 | 2618.07 | 2615.44 | – |
| 83 | $0.92(3\omega_3)$ | 2632.16 | 2629.73 | 2630.66 | 2629.39 | – |
| 84 | $0.82(\omega_{11} + \omega_8)$, $0.42(\omega_7 + \omega_{10})$ | 2643.26 | 2640.40 | 2641.45 | 2640.00 | – |
| 85 | $0.84(\omega_{11} + \omega_7)$ | 2643.47 | 2640.69 | 2641.75 | 2640.33 | – |
| 86 | $0.88(\omega_4 + 2\omega_2)$ | 2650.94 | 2646.22 | 2647.62 | 2645.25 | – |
| 87 | $0.84(\omega_3 + \omega_4 + \omega_1)$ | 2680.09 | 2675.27 | 2677.39 | 2674.51 | – |

| | | | | | | |
|---|---|---|---|---|---|---|
| 88 | $0.42(\omega_3 + \omega_4 + \omega_1)$, $0.79(2\omega_1 + \omega_5)$ | 2696.78 | 2691.79 | 2694.08 | 2691.00 | – |
| 89 | $0.87(\omega_6 + 2\omega_1)$ | 2701.39 | 2696.72 | 2698.65 | 2695.86 | – |
| 90 | $0.89(\omega_3 + \omega_4 + \omega_2)$ | 2704.80 | 2700.39 | 2702.05 | 2699.64 | – |
| 91 | $0.76(\omega_8 + 2\omega_1)$, $0.44(\omega_6 + \omega_1 + \omega_2)$ | 2715.27 | 2709.89 | 2712.05 | 2708.93 | – |
| 92 | $0.85(\omega_1 + \omega_5 + \omega_2)$ | 2724.79 | 2719.93 | 2721.93 | 2719.05 | – |
| 93 | $0.46(\omega_8 + 2\omega_1)$, $0.77(\omega_6 + \omega_1 + \omega_2)$ | 2732.11 | 2727.21 | 2728.99 | 2726.33 | – |
| 94 | $0.89(\omega_7 + 2\omega_1)$ | 2737.54 | 2733.63 | 2735.50 | 2733.09 | – |
| 95 | $0.93(\omega_9 + \omega_{10})$ | 2739.00 | 2736.72 | 2737.69 | 2736.44 | – |
| 96 | $0.66(\omega_8 + \omega_1 + \omega_2)$, $0.59(\omega_6 + 2\omega_2)$ | 2748.59 | 2743.29 | 2744.92 | 2742.19 | – |
| 97 | $0.87(\omega_7 + \omega_1 + \omega_2)$ | 2754.98 | 2750.71 | 2752.38 | 2750.01 | – |
| 98 | $0.65(\omega_8 + \omega_1 + \omega_2)$, $0.61(\omega_6 + 2\omega_2)$ | 2761.77 | 2756.89 | 2758.33 | 2755.85 | – |
| 99 | $0.85(\omega_5 + 2\omega_2)$ | 2763.61 | 2759.67 | 2761.00 | 2758.99 | – |
| 100 | $0.88(2\omega_3 + \omega_4)$ | 2763.99 | 2760.27 | 2761.78 | 2759.74 | – |
| 101 | $0.88(\omega_{11} + \omega_9)$ | 2765.21 | 2762.65 | 2763.63 | 2762.30 | – |
| 102 | $0.88(\omega_7 + 2\omega_2)$ | 2779.11 | 2774.89 | 2776.31 | 2774.12 | – |
| 103 | $0.88(\omega_3 + \omega_1 + \omega_5)$ | 2786.90 | 2782.78 | 2784.61 | 2782.20 | – |
| 104 | $0.91(\omega_6 + \omega_3 + \omega_1)$ | 2788.29 | 2784.23 | 2786.09 | 2783.64 | – |
| 105 | $0.92(\omega_8 + 2\omega_2)$ | 2793.31 | 2789.56 | 2790.87 | 2788.94 | – |
| 106 | $0.56(\omega_6 + \omega_3 + \omega_2)$, $0.72(\omega_3 + \omega_8 + \omega_1)$ | 2807.03 | 2802.37 | 2804.18 | 2801.60 | – |
| 107 | $0.59(\omega_3 + \omega_7 + \omega_1)$, $0.72(\omega_3 + \omega_5 + \omega_2)$ | 2814.67 | 2810.54 | 2812.16 | 2809.92 | – |
| 108 | $0.70(\omega_6 + \omega_3 + \omega_2)$, $0.59(\omega_3 + \omega_8 + \omega_1)$ | 2816.47 | 2812.14 | 2813.72 | 2811.39 | – |
| 109 | $0.93(2\omega_4 + \omega_1)$ | 2819.08 | 2814.26 | 2816.34 | 2813.41 | – |

| | | | | | | |
|---|---|---|---|---|---|---|
| 110 | $0.75(\omega_3 + \omega_7 + \omega_1)$, | 2819.14 | 2815.31 | 2816.86 | 2814.79 | – |
| | $0.57(\omega_3 + \omega_5 + \omega_2)$ | | | | | |
| 111 | $0.91(\omega_3 + \omega_7 + \omega_2)$ | 2836.09 | 2832.08 | 2833.48 | 2831.43 | – |
| 112 | $0.91(2\omega_4 + \omega_2)$ | 2844.60 | 2840.93 | 2841.67 | 2839.19 | – |
| 113 | $0.93(\omega_3 + \omega_8 + \omega_2)$ | 2844.62 | 2840.05 | 2842.34 | 2840.40 | – |
| 114 | $0.88(\omega_9 + 2\omega_1)$ | 2855.35 | 2851.24 | 2852.81 | 2850.59 | – |
| 115 | $0.92(\omega_6 + 2\omega_3)$ | 2874.46 | 2871.18 | 2872.42 | 2870.69 | – |
| 116 | $0.93(2\omega_3 + \omega_5)$ | 2875.50 | 2872.05 | 2873.45 | 2871.59 | – |
| 117 | $0.89(\omega_9 + \omega_1 + \omega_2)$ | 2876.05 | 2871.99 | 2873.54 | 2871.34 | – |
| 118 | $0.93(2\omega_3 + \omega_7)$ | 2897.30 | 2894.00 | 2895.35 | 2893.58 | – |
| 119 | $0.93(2\omega_3 + \omega_8)$ | 2900.85 | 2897.57 | 2898.89 | 2897.12 | – |
| 120 | $0.87(\omega_3 + 2\omega_4)$ | 2901.71 | 2897.51 | 2899.21 | 2896.84 | – |
| 121 | $0.83(\omega_9 + 2\omega_2)$ | 2904.27 | 2900.57 | 2901.65 | 2899.85 | – |
| 122 | $0.68(\omega_{12})$, | 2910.11 | 2907.60 | 2908.61 | 2907.10 | – |
| | $0.55(\omega_{11} + \omega_{10})$ | | | | | |
| 123 | $0.45(\omega_{13})$, | 2915.59 | 2912.31 | 2913.56 | 2911.36 | – |
| | $0.45(2\omega_{10})$, | | | | | |
| | $0.55(\omega_4 + \omega_1 + \omega_5)$ | | | | | |
| 124 | $0.81(\omega_6 + \omega_4 + \omega_1)$ | 2917.88 | 2912.70 | 2915.06 | 2911.96 | – |
| 125 | $0.37(\omega_{13})$, | 2921.64 | 2917.24 | 2919.27 | 2917.04 | – |
| | $0.54(2\omega_{10})$, | | | | | |
| | $0.57(\omega_4 + \omega_1 + \omega_5)$ | | | | | |
| 126 | $0.89(\omega_9 + \omega_3 + \omega_1)$ | 2933.57 | 2929.62 | 2931.20 | 2929.00 | – |
| 127 | $0.71(\omega_6 + \omega_4 + \omega_2)$, | 2939.44 | 2933.32 | 2935.55 | 2932.15 | – |
| | $0.49(\omega_8 + \omega_4 + \omega_1)$ | | | | | |
| 128 | $0.74(\omega_4 + \omega_7 + \omega_1)$, | 2944.01 | 2938.30 | 2940.51 | 2937.28 | – |
| | $0.46(\omega_4 + \omega_5 + \omega_2)$ | | | | | |
| 129 | $0.49(\omega_6 + \omega_4 + \omega_2)$, | 2950.75 | 2945.12 | 2947.26 | 2944.13 | – |
| | $0.77(\omega_8 + \omega_4 + \omega_1)$ | | | | | |

| | | | | | | |
|---|---|---|---|---|---|---|
| 130 | $0.51(\omega_4 + \omega_7 + \omega_1)$, $0.77(\omega_4 + \omega_5 + \omega_2)$ | 2952.92 | 2947.73 | 2949.65 | 2946.88 | – |
| 131 | $0.86(\omega_9 + \omega_3 + \omega_2)$ | 2956.07 | 2952.57 | 2953.82 | 2951.97 | – |
| 132 | $0.52(\omega_{13})$, $0.32(2\omega_{11})$, $0.62(2\omega_{10})$ | 2956.43 | 2953.48 | 2954.65 | 2952.96 | – |
| 133 | $0.82(\omega_4 + \omega_7 + \omega_2)$ | 2969.37 | 2964.55 | 2966.33 | 2963.75 | – |
| 134 | $0.93(\omega_8 + \omega_4 + \omega_2)$ | 2984.46 | 2980.11 | 2981.81 | 2979.39 | – |
| 135 | $0.53(\omega_{12})$, $0.64(\omega_{11} + \omega_{10})$, $0.36(2\omega_1 + \omega_{10})$ | 2994.75 | 2991.02 | 2992.50 | 2990.30 | – |
| 136 | $0.37(\omega_{13})$, $0.73(2\omega_{11})$ | 2999.82 | 2995.74 | 2997.29 | 2994.92 | – |
| 137 | $0.88(\omega_6 + \omega_3 + \omega_4)$ | 3001.82 | 2997.48 | 2999.26 | 2996.80 | – |
| 138 | $0.73(\omega_3 + \omega_4 + \omega_5)$, $0.44(\omega_1 + 2\omega_5)$ | 3006.19 | 3000.76 | 3002.94 | 2999.73 | – |
| 139 | $0.85(\omega_9 + 2\omega_3)$ | 3012.27 | 3009.16 | 3010.27 | 3008.61 | – |
| 140 | $0.53(\omega_3 + \omega_4 + \omega_5)$, $0.45(\omega_1 + 2\omega_5)$, $0.54(2\omega_6 + \omega_1)$ | 3015.71 | 3009.18 | 3011.88 | 3008.22 | – |
| 141 | $0.83(\omega_6 + \omega_1 + \omega_5)$ | 3022.67 | 3016.93 | 3019.58 | 3015.99 | – |
| 142 | $0.88(\omega_3 + \omega_4 + \omega_7)$ | 3026.55 | 3022.13 | 3023.97 | 3021.48 | – |
| 143 | $0.85(\omega_{14})$ | 3028.63 | 3026.39 | 3027.20 | 3025.93 | – |
| 144 | $0.63(\omega_1 + 2\omega_5)$, $0.62(2\omega_6 + \omega_1)$ | 3033.51 | 3028.21 | 3030.28 | 3027.29 | – |
| 145 | $0.45(\omega_8 + \omega_1 + \omega_5)$, $0.79(\omega_3 + \omega_8 + \omega_4)$ | 3037.47 | 3032.86 | 3034.75 | 3032.04 | – |
| 146 | $0.32(\omega_{11} + \omega_{10})$, $0.53(\omega_6 + \omega_8 + \omega_1)$, $0.56(2\omega_1 + \omega_{10})$ | 3038.24 | 3032.67 | 3035.02 | 3031.72 | – |

| | | | | | | |
|---|---|---|---|---|---|---|
| 147 | $0.81(\omega_{15})$ | 3040.89 | 3038.19 | 3039.23 | 3037.67 | – |
| 148 | $0.93(3\omega_4)$ | 3044.72 | 3040.73 | 3042.45 | 3040.12 | – |
| 149 | $0.37(2\omega_1 + \omega_{10})$, $0.73(2\omega_6 + \omega_2)$ | 3045.87 | 3040.40 | 3042.67 | 3039.33 | – |
| 150 | $0.66(\omega_8 + \omega_1 + \omega_5)$, $0.49(\omega_3 + \omega_8 + \omega_4)$ | 3046.57 | 3040.59 | 3042.71 | 3039.61 | – |
| 151 | $0.80(\omega_7 + \omega_1 + \omega_5)$ | 3053.72 | 3048.24 | 3050.52 | 3047.38 | – |
| 152 | $0.44(\omega_6 + \omega_7 + \omega_1)$, $0.70(\omega_6 + \omega_5 + \omega_2)$ | 3055.78 | 3050.39 | 3052.43 | 3049.34 | – |
| 153 | $0.80(\omega_6 + \omega_7 + \omega_1)$ | 3058.83 | 3053.48 | 3055.65 | 3052.56 | – |
| 154 | $0.63(\omega_6 + \omega_8 + \omega_1)$, $0.51(2\omega_1 + \omega_{10})$, $0.33(2\omega_6 + \omega_2)$ | 3063.79 | 3058.42 | 3060.63 | 3057.58 | – |
| 155 | $0.58(\omega_{11} + 2\omega_1)$, $0.33(4\omega_1)$, $0.42(\omega_8 + \omega_1 + \omega_5)$, $0.36(\omega_6 + \omega_5 + \omega_2)$ | 3066.94 | 3062.71 | 3063.64 | 3060.45 | – |
| 156 | $0.84(2\omega_5 + \omega_2)$ | 3067.22 | 3061.47 | 3064.36 | 3062.08 | – |
| 157 | $0.44(\omega_6 + \omega_8 + \omega_2)$, $0.34(2\omega_8 + \omega_1)$, $0.68(\omega_1 + \omega_{10} + \omega_2)$ | 3068.47 | 3062.83 | 3064.97 | 3061.86 | – |
| 158 | $0.67(\omega_8 + \omega_7 + \omega_1)$, $0.58(\omega_6 + \omega_7 + \omega_2)$ | 3072.93 | 3067.54 | 3069.48 | 3066.22 | – |
| 159 | $0.76(2\omega_8 + \omega_1)$, $0.40(\omega_1 + \omega_{10} + \omega_2)$ | 3073.72 | 3067.39 | 3069.72 | 3066.66 | – |
| 160 | $0.83(\omega_9 + \omega_4 + \omega_1)$ | 3078.45 | 3073.50 | 3075.56 | 3072.69 | – |
| 161 | $0.51(\omega_8 + \omega_5 + \omega_2)$, $0.47(\omega_6 + \omega_7 + \omega_2)$, $0.54(\omega_{11} + \omega_1 + \omega_2)$ | 3084.26 | 3079.09 | 3080.67 | 3077.35 | – |

| | | | | | | |
|---|---|---|---|---|---|---|
| 162 | $0.68(\omega_7 + \omega_5 + \omega_2)$, $0.44(2\omega_7 + \omega_1)$ | 3084.89 | 3078.59 | 3081.04 | 3078.22 | – |
| 163 | $0.60(\omega_8 + \omega_7 + \omega_1)$, $0.49(\omega_6 + \omega_7 + \omega_2)$, $0.36(\omega_{11} + \omega_1 + \omega_2)$ | 3088.19 | 3083.61 | 3084.80 | 3081.97 | – |
| 164 | $0.83(2\omega_7 + \omega_1)$ | 3088.46 | 3082.91 | 3085.52 | 3082.99 | – |
| 165 | $0.79(\omega_6 + \omega_8 + \omega_2)$, $0.41(\omega_1 + \omega_{10} + \omega_2)$ | 3096.49 | 3091.53 | 3093.38 | 3090.72 | – |
| 166 | $0.72(\omega_8 + \omega_5 + \omega_2)$, $0.55(\omega_{11} + \omega_1 + \omega_2)$ | 3103.38 | 3099.18 | 3099.94 | 3097.05 | – |
| 167 | $0.90(2\omega_7 + \omega_2)$ | 3103.49 | 3097.96 | 3100.80 | 3098.55 | – |
| 168 | $0.46(\omega_7 + \omega_5 + \omega_2)$, $0.77(\omega_9 + \omega_4 + \omega_2)$ | 3104.76 | 3100.05 | 3101.90 | 3099.26 | – |
| 169 | $0.43(\omega_3 + 2\omega_5)$, $0.80(2\omega_6 + \omega_3)$ | 3110.52 | 3105.80 | 3107.60 | 3105.02 | – |
| 170 | $0.90(\omega_{10} + 2\omega_2)$ | 3110.84 | 3106.91 | 3108.28 | 3106.22 | – |
| 171 | $0.92(\omega_8 + \omega_7 + \omega_2)$ | 3112.40 | 3108.13 | 3109.89 | 3107.48 | – |
| 172 | $0.88(\omega_6 + \omega_3 + \omega_5)$ | 3116.51 | 3112.06 | 3113.82 | 3111.38 | – |
| 173 | $0.93(2\omega_8 + \omega_2)$ | 3120.27 | 3116.68 | 3118.11 | 3116.17 | – |
| 174 | $0.83(\omega_3 + 2\omega_5)$, $0.44(2\omega_6 + \omega_3)$ | 3123.08 | 3119.33 | 3120.82 | 3118.81 | – |
| 175 | $0.77(\omega_3 + \omega_1 + \omega_{10})$, $0.43(\omega_6 + \omega_3 + \omega_8)$ | 3127.83 | 3122.67 | 3124.62 | 3121.84 | – |
| 176 | $0.83(\omega_{11} + 2\omega_2)$ | 3131.99 | 3126.22 | 3127.20 | 3124.65 | – |
| 177 | $0.88(\omega_6 + 2\omega_4)$ | 3134.57 | 3129.05 | 3131.22 | 3128.05 | – |
| 178 | $0.77(\omega_3 + \omega_7 + \omega_5)$, $0.42(\omega_9 + \omega_3 + \omega_4)$ | 3141.60 | 3136.64 | 3138.47 | 3135.87 | – |
| 179 | $0.48(\omega_6 + \omega_3 + \omega_7)$, $0.64(\omega_3 + \omega_8 + \omega_5)$, $0.44(\omega_{11} + \omega_3 + \omega_1)$ | 3142.35 | 3137.73 | 3139.61 | 3136.85 | – |

| | | | | | | |
|---|---|---|---|---|---|---|
| 180 | $0.79(\omega_6 + \omega_3 + \omega_7)$, | 3143.64 | 3138.82 | 3140.87 | 3138.29 | – |
| | $0.42(\omega_3 + \omega_8 + \omega_5)$ | | | | | |
| 181 | $0.88(2\omega_4 + \omega_5)$ | 3144.50 | 3139.35 | 3141.54 | 3138.49 | – |
| 182 | $0.49(\omega_3 + \omega_1 + \omega_{10})$, | 3151.96 | 3147.54 | 3149.37 | 3146.94 | – |
| | $0.79(\omega_6 + \omega_3 + \omega_8)$ | | | | | |
| 183 | $0.49(\omega_3 + \omega_7 + \omega_5)$, | 3159.33 | 3154.89 | 3156.59 | 3154.19 | – |
| | $0.71(\omega_9 + \omega_3 + \omega_4)$ | | | | | |
| 184 | $0.85(2\omega_4 + \omega_7)$ | 3160.20 | 3154.63 | 3156.97 | 3153.69 | – |
| 185 | $0.53(\omega_3 + \omega_8 + \omega_5)$, | 3161.88 | 3156.27 | 3158.63 | 3155.44 | – |
| | $0.70(\omega_{11} + \omega_3 + \omega_1)$ | | | | | |
| 186 | $0.80(\omega_3 + 2\omega_7)$, | 3164.72 | 3160.87 | 3162.41 | 3160.33 | – |
| | $0.45(\omega_3 + \omega_{10} + \omega_2)$ | | | | | |
| 187 | $0.44(\omega_3 + 2\omega_7)$, | 3165.36 | 3161.40 | 3162.95 | 3160.82 | – |
| | $0.81(\omega_3 + \omega_{10} + \omega_2)$ | | | | | |
| 188 | $0.94(\omega_3 + \omega_8 + \omega_7)$ | 3168.55 | 3164.61 | 3166.28 | 3164.09 | – |
| 189 | $0.79(4\omega_1)$ | 3171.12 | 3167.62 | 3167.79 | 3163.26 | – |
| 190 | $0.91(\omega_3 + 2\omega_8)$ | 3173.88 | 3165.45 | 3169.11 | 3167.15 | – |
| 191 | $0.85(\omega_9 + \omega_1 + \omega_5)$ | 3175.50 | 3170.13 | 3172.33 | 3169.19 | – |
| 192 | $0.87(\omega_9 + \omega_6 + \omega_1)$ | 3178.91 | 3173.60 | 3175.76 | 3172.68 | – |
| 193 | $0.94(\omega_8 + 2\omega_4)$ | 3181.83 | 3177.51 | 3179.28 | 3176.82 | – |
| 194 | $0.86(\omega_{11} + \omega_3 + \omega_2)$ | 3187.19 | 3182.12 | 3183.76 | 3181.06 | – |
| 195 | $0.86(3\omega_1 + \omega_2)$ | 3197.27 | 3191.75 | 3192.18 | 3187.44 | – |
| 196 | $0.51(\omega_9 + \omega_6 + \omega_2)$, | 3198.00 | 3189.61 | 3193.89 | 3190.78 | – |
| | $0.70(\omega_9 + \omega_8 + \omega_1)$ | | | | | |
| 197 | $0.75(\omega_9 + \omega_5 + \omega_2)$, | 3205.08 | 3200.30 | 3202.16 | 3199.48 | – |
| | $0.47(\omega_9 + \omega_7 + \omega_1)$ | | | | | |
| 198 | $0.68(\omega_9 + \omega_6 + \omega_2)$, | 3206.11 | 3201.03 | 3202.96 | 3200.15 | – |
| | $0.55(\omega_9 + \omega_8 + \omega_1)$ | | | | | |
| 199 | $0.46(\omega_9 + \omega_5 + \omega_2)$, | 3210.44 | 3205.96 | 3207.74 | 3205.19 | – |
| | $0.77(\omega_9 + \omega_7 + \omega_1)$ | | | | | |

| | | | | | | |
|---|---|---|---|---|---|---|
| 200 | $0.85(2\omega_1 + 2\omega_2)$ | 3224.76 | 3221.38 | 3218.48 | 3214.59 | – |

## S4. NAPHTHALENE

TABLE S4: 128 lowest-energy states of naphthalene computed with VHCI and VHCI+PT2. Excited states are reported relative to the ZPE. Calculated using the quartic PES from Ref. 7. Multiple assignments are given when the CI wavefunction weight differs by less than a factor of two. Assignments use the mode-numbering convention of Ref. 7 and are taken from the $\varepsilon_1$ = 1 cm$^{-1}$ calculation, while the $\varepsilon_1$ = 1.5 cm$^{-1}$ data is presented in order of energy. All energies are in cm$^{-1}$.

| | | $\varepsilon_1 = 1.5$ | | $\varepsilon_1 = 1$ | |
|---|---|---|---|---|---|
| | Assignment | Var | $\varepsilon_2 = 0.2$ | Var | $\varepsilon_2 = 0.2$ |
| 1 | ZPE | 31772.71 | 31764.77 | 31769.90 | 31764.34 |
| 2 | $0.94(\omega_{48})$ | 168.17 | 165.20 | 166.89 | 164.63 |
| 3 | $0.94(\omega_{13})$ | 182.57 | 179.28 | 181.28 | 178.79 |
| 4 | $0.94(2\omega_{48})$ | 335.22 | 329.48 | 333.17 | 328.69 |
| 5 | $0.94(\omega_{13} + \omega_{48})$ | 349.25 | 342.84 | 346.48 | 341.76 |
| 6 | $0.94(\omega_{24})$ | 358.59 | 356.26 | 357.83 | 355.97 |
| 7 | $0.94(2\omega_{13})$ | 362.91 | 357.23 | 360.75 | 356.49 |
| 8 | $0.94(\omega_{16})$ | 392.38 | 389.05 | 391.19 | 388.64 |
| 9 | $0.94(\omega_{28})$ | 468.62 | 464.50 | 467.08 | 463.93 |
| 10 | $0.94(\omega_{47})$ | 477.41 | 472.97 | 475.83 | 472.45 |
| 11 | $0.94(3\omega_{48})$ | 503.57 | 493.98 | 499.45 | 492.38 |
| 12 | $0.94(\omega_{44})$ | 510.13 | 507.21 | 509.14 | 506.90 |
| 13 | $0.94(\omega_{13} + 2\omega_{48})$ | 520.21 | 508.45 | 513.76 | 505.56 |
| 14 | $0.92(\omega_9)$ | 516.63 | 513.90 | 515.71 | 513.90 |
| 15 | $0.94(\omega_{24} + \omega_{48})$ | 525.51 | 520.66 | 524.19 | 520.17 |
| 16 | $0.94(2\omega_{13} + \omega_{48})$ | 531.70 | 521.25 | 527.40 | 519.62 |

| | | | | | |
|---|---|---|---|---|---|
| 17 | $0.95(\omega_{13} + \omega_{24})$ | 540.25 | 534.44 | 538.23 | 533.80 |
| 18 | $0.94(3\omega_{13})$ | 547.30 | 537.32 | 543.63 | 536.16 |
| 19 | $0.94(\omega_{16} + \omega_{48})$ | 559.84 | 553.66 | 557.45 | 552.91 |
| 20 | $0.95(\omega_{13} + \omega_{16})$ | 574.95 | 567.82 | 572.18 | 566.97 |
| 21 | $0.94(\omega_{36})$ | 627.52 | 624.15 | 626.59 | 623.88 |
| 22 | $0.94(\omega_{12})$ | 627.10 | 623.25 | 625.90 | 622.90 |
| 23 | $0.93(\omega_{28} + \omega_{48})$ | 637.29 | 628.93 | 634.10 | 627.78 |
| 24 | $0.94(\omega_{47} + \omega_{48})$ | 644.59 | 637.60 | 641.96 | 636.76 |
| 25 | $0.94(\omega_{13} + \omega_{28})$ | 650.39 | 642.60 | 648.20 | 642.05 |
| 26 | $0.94(\omega_{13} + \omega_{47})$ | 660.18 | 651.61 | 655.64 | 649.89 |
| 27 | $0.93(4\omega_{48})$ | 673.04 | 658.86 | 667.42 | 656.86 |
| 28 | $0.94(\omega_{44} + \omega_{48})$ | 679.55 | 673.20 | 677.46 | 672.57 |
| 29 | $0.93(\omega_{13} + 3\omega_{48})$ | 687.47 | 681.09 | 680.63 | 668.98 |
| 30 | $0.93(\omega_{9} + \omega_{48})$ | 687.62 | 671.98 | 685.30 | 680.46 |
| 31 | $0.94(\omega_{13} + \omega_{44})$ | 693.22 | 686.75 | 691.10 | 686.14 |
| 32 | $0.94(\omega_{24} + 2\omega_{48})$ | 695.49 | 686.19 | 692.10 | 685.02 |
| 33 | $0.94(2\omega_{13} + 2\omega_{48})$ | 699.43 | 684.49 | 693.31 | 681.98 |
| 34 | $0.93(\omega_{9} + \omega_{13})$ | 700.49 | 694.04 | 698.36 | 693.44 |
| 35 | $0.93(\omega_{15})$ | 703.34 | 694.91 | 700.49 | 693.82 |
| 36 | $0.94(\omega_{13} + \omega_{24} + \omega_{48})$ | 709.25 | 699.45 | 706.09 | 698.47 |
| 37 | $0.94(3\omega_{13} + \omega_{48})$ | 714.24 | 699.73 | 708.00 | 697.25 |
| 38 | $0.94(2\omega_{24})$ | 716.75 | 711.91 | 715.36 | 711.55 |
| 39 | $0.95(2\omega_{13} + \omega_{24})$ | 721.69 | 712.97 | 718.67 | 712.04 |
| 40 | $0.94(4\omega_{13})$ | 726.80 | 714.61 | 722.35 | 713.17 |
| 41 | $0.94(\omega_{16} + 2\omega_{48})$ | 731.14 | 719.81 | 726.94 | 718.44 |
| 42 | $0.94(\omega_{13} + \omega_{16} + \omega_{48})$ | 745.04 | 733.12 | 740.64 | 731.65 |
| 43 | $0.95(\omega_{16} + \omega_{24})$ | 749.65 | 744.10 | 747.85 | 743.63 |
| 44 | $0.95(2\omega_{13} + \omega_{16})$ | 757.20 | 746.68 | 753.28 | 745.43 |
| 45 | $0.89(\omega_{8})$ | 760.75 | 756.84 | 759.60 | 756.59 |
| 46 | $0.93(\omega_{46})$ | 771.82 | 764.84 | 769.58 | 763.94 |

| | | | | | |
|---|---|---|---|---|---|
| 47 | $0.94(\omega_{27})$ | 774.88 | 769.48 | 772.98 | 768.86 |
| 48 | $0.93(2\omega_{16})$ | 784.60 | 778.43 | 782.34 | 777.86 |
| 49 | $0.94(\omega_{12} + \omega_{48})$ | 794.89 | 787.48 | 792.25 | 786.57 |
| 50 | $0.95(\omega_{36} + \omega_{48})$ | 795.06 | 788.83 | 793.07 | 788.27 |
| 51 | $0.94(\omega_{23})$ | 797.26 | 793.29 | 796.15 | 793.00 |
| 52 | $0.92(\omega_{28} + 2\omega_{48})$ | 806.14 | 793.60 | 800.91 | 791.30 |
| 53 | $0.94(\omega_{12} + \omega_{13})$ | 808.89 | 801.54 | 806.44 | 800.77 |
| 54 | $0.95(\omega_{13} + \omega_{36})$ | 809.44 | 803.09 | 807.46 | 802.55 |
| 55 | $0.94(\omega_{47} + 2\omega_{48})$ | 815.02 | 803.49 | 810.24 | 801.78 |
| 56 | $0.93(\omega_{13} + \omega_{28} + \omega_{48})$ | 820.52 | 807.54 | 815.56 | 805.45 |
| 57 | $0.78(\omega_{11})$, $0.52(\omega_{13} + \omega_{47} + \omega_{48})$ | 825.91 | 818.15 | 822.82 | 816.30 |
| 58 | $0.94(\omega_{24} + \omega_{28})$ | 826.24 | 819.94 | 824.18 | 819.29 |
| 59 | $0.52(\omega_{11})$, $0.78(\omega_{13} + \omega_{47} + \omega_{48})$ | 830.50 | 818.05 | 826.04 | 818.32 |
| 60 | $0.94(2\omega_{13} + \omega_{28})$ | 832.83 | 821.32 | 828.23 | 819.47 |
| 61 | $0.94(\omega_{24} + \omega_{47})$ | 833.95 | 827.44 | 832.04 | 826.92 |
| 62 | $0.92(5\omega_{48})$ | 842.14 | 829.85 | 835.56 | 820.85 |
| 63 | $0.94(2\omega_{13} + \omega_{47})$ | 847.23 | 838.05 | 837.11 | 828.20 |
| 64 | $0.94(\omega_{44} + 2\omega_{48})$ | 850.09 | 825.73 | 843.68 | 836.78 |
| 65 | $0.92(\omega_{9} + 2\omega_{48})$ | 856.03 | 846.81 | 852.61 | 845.77 |
| 66 | $0.93(\omega_{13} + 4\omega_{48})$ | 861.25 | 851.42 | 856.18 | 835.43 |
| 67 | $0.93(\omega_{24} + 3\omega_{48})$ | 861.35 | 853.82 | 857.47 | 848.14 |
| 68 | $0.93(\omega_{13} + \omega_{44} + \omega_{48})$ | 862.08 | 849.83 | 857.86 | 850.27 |
| 69 | $0.94(\omega_{16} + \omega_{28})$ | 866.76 | 857.25 | 858.50 | 852.81 |
| 70 | $0.93(2\omega_{13} + 3\omega_{48})$ | 867.92 | 861.29 | 860.55 | 844.94 |
| 71 | $0.83(\omega_{15} + \omega_{48})$ | 868.88 | 848.30 | 862.89 | 853.35 |
| 72 | $0.92(\omega_{24} + \omega_{44})$ | 869.43 | 859.66 | 865.95 | 861.98 |
| 73 | $0.92(\omega_{9} + \omega_{13} + \omega_{48})$ | 871.18 | 862.22 | 865.97 | 858.51 |
| 74 | $0.85(\omega_{16} + \omega_{47})$ | 873.76 | 864.97 | 867.93 | 861.14 |

| | | | | | |
|---|---|---|---|---|---|
| 75 | $0.93(2\omega_{13} + \omega_{44})$ | 874.34 | 869.55 | 870.42 | 863.86 |
| 76 | $0.94(\omega_{13} + \omega_{24} + 2\omega_{48})$ | 876.43 | 870.20 | 871.68 | 861.21 |
| 77 | $0.92(\omega_{9} + \omega_{24})$ | 876.72 | 863.08 | 872.93 | 869.19 |
| 78 | $0.93(\omega_{26})$ | 880.87 | 872.32 | 874.30 | 869.42 |
| 79 | $0.92(\omega_{13} + \omega_{15})$ | 881.66 | 869.30 | 876.99 | 867.29 |
| 80 | $0.93(\omega_{9} + 2\omega_{13})$ | 884.08 | 876.55 | 877.84 | 871.45 |
| 81 | $0.94(2\omega_{24} + \omega_{48})$ | 889.18 | 876.34 | 881.80 | 875.88 |
| 82 | $0.94(2\omega_{13} + \omega_{24} + \omega_{48})$ | 897.03 | 889.60 | 884.85 | 874.82 |
| 83 | $0.93(\omega_{16} + 3\omega_{48})$ | 899.28 | 884.11 | 893.63 | 882.36 |
| 84 | $0.95(\omega_{13} + 2\omega_{24})$ | 901.35 | 890.20 | 894.78 | 888.97 |
| 85 | $0.94(3\omega_{13} + \omega_{24})$ | 901.75 | 895.96 | 897.63 | 889.01 |
| 86 | $0.94(\omega_{16} + \omega_{44})$ | 908.71 | 902.84 | 899.94 | 895.48 |
| 87 | $0.93(\omega_{9} + \omega_{16})$ | 913.70 | 897.31 | 906.81 | 902.35 |
| 88 | $0.94(\omega_{13} + \omega_{16} + 2\omega_{48})$ | 926.08 | 910.55 | 907.93 | 895.33 |
| 89 | $0.94(2\omega_{13} + \omega_{16} + \omega_{48})$ | 929.16 | 922.25 | 920.53 | 908.71 |
| 90 | $0.95(\omega_{16} + \omega_{24} + \omega_{48})$ | 931.04 | 922.20 | 921.20 | 909.64 |
| 91 | $0.90(\omega_{8} + \omega_{48})$ | 934.02 | 926.81 | 926.99 | 921.55 |
| 92 | $0.95(\omega_{13} + \omega_{16} + \omega_{24})$ | 935.40 | 924.38 | 928.49 | 921.45 |
| 93 | $0.85(\omega_{46} + \omega_{48})$ | 937.67 | 930.10 | 930.87 | 922.01 |
| 94 | $0.93(\omega_{14})$ | 941.33 | 933.02 | 931.51 | 925.86 |
| 95 | $0.87(2\omega_{28})$ | 944.22 | 937.41 | 934.94 | 929.18 |
| 96 | $0.91(\omega_{27} + \omega_{48})$ | 944.48 | 938.50 | 938.44 | 932.06 |
| 97 | $0.91(\omega_{8} + \omega_{13})$ | 946.16 | 937.50 | 942.03 | 936.69 |
| 98 | $0.67(\omega_{43})$, $0.65(\omega_{13} + \omega_{46})$ | 954.16 | 946.01 | 942.27 | 937.02 |
| 99 | $0.91(\omega_{28} + \omega_{47})$ | 954.34 | 945.74 | 942.94 | 936.52 |
| 100 | $0.93(2\omega_{16} + \omega_{48})$ | 954.53 | 944.88 | 950.64 | 942.81 |
| 101 | $0.94(2\omega_{47})$ | 954.99 | 946.58 | 951.25 | 945.22 |
| 102 | $0.66(\omega_{43})$, $0.65(\omega_{13} + \omega_{46})$ | 955.10 | 947.82 | 951.54 | 946.21 |

| | | | | | |
|---|---|---|---|---|---|
| 103 | $0.93(\omega_{13} + \omega_{27})$ | 962.87 | 954.43 | 951.87 | 945.52 |
| 104 | $0.93(\omega_{45})$ | 965.22 | 955.12 | 952.82 | 947.28 |
| 105 | $0.69(\omega_{10})$, $0.63(\omega_{12} + 2\omega_{48})$ | 966.40 | 959.60 | 959.38 | 952.49 |
| 106 | $0.63(\omega_{10})$, $0.69(\omega_{12} + 2\omega_{48})$ | 968.92 | 961.50 | 962.02 | 955.87 |
| 107 | $0.93(\omega_{23} + \omega_{48})$ | 976.77 | 967.10 | 964.35 | 958.97 |
| 108 | $0.92(\omega_{25})$ | 977.70 | 966.14 | 966.09 | 960.24 |
| 109 | $0.94(\omega_{12} + \omega_{13} + \omega_{48})$ | 978.08 | 971.77 | 973.57 | 964.56 |
| 110 | $0.95(\omega_{13} + \omega_{36} + \omega_{48})$ | 978.99 | 972.19 | 973.61 | 966.08 |
| 111 | $0.94(\omega_{28} + \omega_{44})$ | 982.41 | 977.49 | 976.06 | 971.08 |
| 112 | $0.93(\omega_{47} + 3\omega_{48})$ | 982.93 | 967.73 | 976.85 | 965.69 |
| 113 | $0.94(\omega_{13} + \omega_{23})$ | 984.01 | 978.50 | 976.88 | 971.60 |
| 114 | $0.94(\omega_{24} + \omega_{36})$ | 984.89 | 978.67 | 981.37 | 977.64 |
| 115 | $0.94(\omega_{12} + \omega_{24})$ | 986.66 | 979.81 | 982.39 | 977.99 |
| 116 | $0.92(\omega_{9} + \omega_{28})$ | 989.29 | 971.43 | 982.83 | 978.03 |
| 117 | $0.94(\omega_{44} + \omega_{47})$ | 993.42 | 982.96 | 984.23 | 979.12 |
| 118 | $0.79(\omega_{11} + \omega_{48})$, $0.48(\omega_{13} + \omega_{47} + 2\omega_{48})$ | 993.93 | 987.08 | 988.34 | 979.28 |
| 119 | $0.93(\omega_{9} + \omega_{47})$ | 1004.86 | 993.98 | 991.49 | 986.44 |
| 120 | $0.48(\omega_{11} + \omega_{48})$, $0.80(\omega_{13} + \omega_{47} + 2\omega_{48})$ | 1011.21 | 994.92 | 992.99 | 981.98 |
| 121 | $0.81(\omega_{11} + \omega_{13})$, $0.43(2\omega_{13} + \omega_{47} + \omega_{48})$ | 1013.18 | 1008.63 | 1000.67 | 991.94 |
| 122 | $0.43(\omega_{11} + \omega_{13})$, $0.83(2\omega_{13} + \omega_{47} + \omega_{48})$ | 1017.51 | 1012.86 | 1005.37 | 994.19 |
| 123 | $0.92(\omega_{35})$ | 1017.62 | 1011.96 | 1011.79 | 1008.21 |
| 124 | $0.94(\omega_{16} + \omega_{36})$ | 1018.41 | 1011.70 | 1015.91 | 1011.51 |
| 125 | $0.94(\omega_{12} + \omega_{16})$ | 1024.79 | 1020.17 | 1016.18 | 1010.98 |
| 126 | $0.93(2\omega_{44})$ | 1028.83 | 1023.98 | 1016.19 | 1012.70 |

| | | | | | |
|---|---|---|---|---|---|
| 127 | $0.94(3\omega_{13} + \omega_{47})$ | 1031.65 | 1027.03 | 1016.56 | 1005.20 |
| 128 | $0.92(\omega_9 + \omega_{44})$ | 1039.82 | 924.03 | 1023.43 | 1019.82 |

## REFERENCES


[1]D. Begue, P. Carbonniere, and C. Pouchan, "Calculations of Vibrational Energy Levels by Using a Hybrid ab Initio and DFT Quartic Force Field: Application to Acetonitrile," J. Phys. Chem. A **109**, 4611–4616 (2005).

[2]R. Garnier, M. Odunlami, V. Le Bris, D. Bégué, I. Baraille, and O. Coulaud, "Adaptive vibrational configuration interaction (A-VCI): A posteriori error estimation to efficiently compute anharmonic IR spectra," J. Chem. Phys. **144**, 1–4 (2016).

[3]T. Delahaye, A. Nikitin, M. Rey, P. G. Szalay, and V. G. Tyuterev, "A new accurate ground-state potential energy surface of ethylene and predictions for rotational and vibrational energy levels," J. Chem. Phys. **141** (2014), 10.1063/1.4894419.

[4]M. Sibaev and D. L. Crittenden, "The PyPES library of high quality semi-global potential energy surfaces," J. Comput. Chem. **36**, 2200–2207 (2015).

[5]D. Bégué, N. Gohaud, C. Pouchan, P. Cassam-Chenaï, and J. Liévin, "A comparison of two methods for selecting vibrational configuration interaction spaces on a heptatomic system: Ethylene oxide," J. Chem. Phys. **127**, 164115 (2007).

[6]M. Odunlami, V. Le Bris, D. Bégué, I. Baraille, and O. Coulaud, "A-VCI: A flexible method to efficiently compute vibrational spectra," J. Chem. Phys. **146**, 214108 (2017).

[7]E. Cané, A. Miani, and A. Trombetti, "Anharmonic force fields of naphthalene-h8 and naphthalene-d 8," J. Phys. Chem. A **111**, 8218–8222 (2007).
